# Supplementary material for: Self-supervised Answer Retrieval on Clinical Notes
Source: arXiv:2108.00775 source file (2021-08-02)
Supplement: Supplementary file 1 [file Appendices.tex]

\begin{table}[h!]
%\begin{SCtable}
\centering
 \begin{tabular}{l c c c} 
 \textbf{Experiment} & \textbf{R@1} & \textbf{R@10} & \textbf{R@32} \\
 \hline
 \hline

\textbf{Precomputed Embeddings} \\
CDV+BioBERT (Replication)                       & 62.36          & 96.0           & \textbf{100} \\
CDV+FastText (Replication)                      & 60.49          & \textbf{98.37} & 99.9 \\
\hline
\textbf{BioBERT Fine-Tuning} \\
CDV+BioBERT FT (Non-Incremental)                & 10.5           & 93.6           & 99.9 \\
CDV+BioBERT FT(Multi-CLS)                       & 49.9           & 94.6           & 99.9 \\
CDV+BioBERT FT(Multi-CLS) + FF-Pool             & 58.4           & 95.4           & 99.9 \\
CDV+BioBERT FT(CLS-Pool) + ELU                  & 64.5           & 96.4           & \textbf{100}  \\ 
CDV+BioBERT FT(CLS) + LAMB-Optim + LR-Decr.     & 61.2           & 98.3           & 99.9 \\

\hline
\textbf{Different Pooling Strategies} \\
CDV+BioBERT 4 Last Layer Pool (256-BLSTM)       & 47.0           & 94.0           & 99.9 \\
CDV+BioBERT 4 Last Layer Pool (512-BLSTM)       & 51.59          & 94.47          & 99.9 \\
CDV+BioBERT AVG-Pool+ELU (512-BLSTM)            & 61.5           & 96.3           & \textbf{100}  \\

\hline
\textbf{Without LSTM} \\
BioBERT AVG without LSTM                        & 50.5           & 94.5           & 99.9 \\

\hline
\textbf{Hierarchical RNN} \\
CDV+FastText (Word GRU + BiLSTM)                & 10.0           & 93.9           & 99.9 \\
CDV+FastText (Word GRU + BiLSTM) + Noise        & 11.31          & 94.99          & 99.9 \\ 

\hline
\textbf{LSTM Replacement with a Transformer} \\
CDV-Transformer CLS-Pool 4-Layer 6-Heads BS64   & 53.3           & 95.0           & 99.9 \\
CDV-Transformer CLS-Pool 6-Layer 8-Heads BS48   & 53.5           & 95.2           & 99.9 \\
CDV-Transformer AVG-Pool 6-Layer 8-Heads BS48   & 58.0           & 95.8           & 99.9 \\
CDV-Transformer FT(CLS-Pool) 4-Layer 6-Heads    & 63.2           & 96.2           & 99.9 \\
CDV-Transformer FT(CLS-Pool) 6-Layer 8-Heads    & 60.4           & 96.1           & 99.9 \\

\end{tabular}

\caption{Hyperparameters}
\label{fig:cdv_enhancements}

%\end{SCtable}
\end{table}
